# Supplementary material for: DiffuseGAE: Controllable and High-fidelity Image Manipulation from Disentangled Representation
Source: arXiv:2307.05899 source file (2023-07-12)
Supplement: Supplementary file 1 [file appendix.tex]

\begin{appendix}

\end{appendix}
